# Supplementary material for: MuscleVAE: Model-Based Controllers of Muscle-Actuated Characters
Source: arXiv:2312.07340 source file (2023-12-12)
Supplement: Supplementary file 1 [file supp_muscle_activation.tex]

\subsection{Muscle Activation Dynamics}
Muscle activation dynamics refer to the series of events and processes that occur from the moment a muscle receives a neural signal (excitation) to the point it generates a mechanical response (activation).

Muscle excitation  refers to the neural signal, or motor neuron input, that stimulates the muscle to contract. When the nervous system sends a signal to a muscle, it doesn't result in an instantaneous force output. Instead, the muscle goes through a process of translating that neural input into a mechanical response. The excitation process can be thought of as the "trigger" that begins the cascade of events leading to muscle contraction.

Once the muscle is excited, a series of biochemical processes ensue, resulting in the muscle generating force. The activation is a time-varying process, which relates to the development of force within the muscle after the excitation signal has been received. This force is not developed instantaneously but takes time to rise to a peak value and then decay, even if the excitation is maintained.

Here is the common formula describing the relationship between excitation and activation. In this section since all the variables, such as action, excitation, activation, and the relation variable \( \beta \), pertain to a specific muscle and even when vectorized they multiply point-by-point, we will ignore the vector nature of these variables for simplification.

\begin{equation}
\dot{\alpha} = \frac{1}{\tau(\epsilon, \alpha)}\left(\epsilon-\alpha\right)
\label{equ:activation_dynamics}
\end{equation}
where the $\epsilon$ denotes the excitation level of muscle, the $\tau(\epsilon, \alpha)$ adjusts the change rate of activation level. A common used case of $\tau(\epsilon, \alpha)$ lies in

\begin{equation}
\tau(\epsilon, \alpha) = 
\begin{cases} 
\tau_1(\alpha)=0.01 \times (0.5 + 1.5 \alpha) & \text{if } \epsilon > \alpha \\
\tau_2(\alpha)=\dfrac{0.04}{0.5 + 1.5 \alpha} & \text{otherwise }
\end{cases}
\label{equ:excitation_tau}
\end{equation}

In a manner akin to activation, excitation also has a numerical range that restricts its values to a specific region, thereby preventing muscles from generating discontinuous mechanical effects. The excitation just like the activation, has certain region $[0, 1]$. Thus, leading to the region of $\dot{\alpha}$,

\begin{equation}
\begin{cases} 
\atv+\tau_1(\atv)\dot{\alpha} \le 1  & \text{if } \epsilon > \alpha, \text{only need to obey when} \ \epsilon \le 1 \\
\atv + \tau_2(\atv)\dot{\alpha} \ge 0 & \text{otherwise,  only need to obey when} \ \epsilon \ge 0
\end{cases}
\label{equ:activation_dot_constraint}
\end{equation}

The discrete form of change rate of activation is 

\begin{equation}
\dot{\alpha} = \frac{\alpha^t-\alpha^{t-1}}{\dt} 
\label{equ:activation_dot}
\end{equation}

Using \eqn \eqref{equ:activation_dot}, we could reach the constraint of current activation's constraint given to the last   activation,

\begin{equation}
\begin{cases} 
\alpha^t \le 1 \ \text{and}\  \alpha^t \le \alpha^{t-1} + \dfrac{\dt(1-\alpha^{t-1} )}{\tau_1(\alpha^{t-1} )}  & \text{if } \epsilon^{t} > \alpha^{t-1} \\
\alpha^t \ge 0 \ \text{and}\  \alpha^t \ge \alpha^{t-1} - \dfrac{\dt\alpha^{t-1} }{\tau_2(\alpha^{t-1} )} & \text{otherwise } 
\end{cases}
\end{equation}

It's easy to find that the right bound $\alpha^{t-1} + \dfrac{\dt(1-\alpha^{t-1} )}{\tau_1(\alpha^{t-1} )}$  is always larger than left bound $\alpha^{t-1} - \dfrac{\dt\alpha^{t-1} }{\tau_2(\alpha^{t-1} )}$and the left bound is always larger than 0 due to the properties of $\tau_1$ and $\tau_2$. So, if we restrict the current activation in the bound of \eqn \eqref{equ:next_activation_constraint}, no matter what last activation came, there will be an excitation value within $[0, 1]$
to reach next frame's activation according to the activation dynamics.

\begin{equation}
\alpha^{t-1} - \dfrac{\dt\alpha^{t-1} }{\tau_2(\alpha^{t-1} )} \le \alpha^{t} \le \text{min}(\alpha^{t-1} + \dfrac{\dt(1-\alpha^{t-1} )}{\tau_1(\alpha^{t-1} )}  , 1.0)
\label{equ:next_activation_constraint}
\end{equation}

We plot the relationship between next activation and last activation given by Equation \eqref{fig:next_activation_constraint} under the situation of 120 simulation Hz. The space between the red solid line (upper bound) and the blue solid line (lower bound) is the valid range of next activation following the activation dynamics.

\begin{figure}
 \includegraphics[width=0.4\textwidth]{Images/act_dyn_constrain.pdf}
 \caption{The constraints depending on last activation corresponding to the muscle activation dynamics at 120Hz. The red solid line represents the right bound, and the dashed line represents the part of right bound of where is greater than 1.0. The blue solid line represents the left bound. The green dashed line is an auxiliary curve, representing $\alpha$.}
 \label{fig:next_activation_constraint}
\end{figure}
